# Supplementary material for: Phase behaviour of active particles in block copolymer melts
Source: arXiv:2203.06495 ancillary file (2022-03-15)
Supplement: Supplementary file 1 [file ESI.pdf]

# Supporting information to:
# Phase behaviour of active particles in block copolymer melts

Javier Diaz
*CECAM, Centre Européen de Calcul Atomique et Moléculaire,
EPFL, École Polytechnique Fédérale de Lausanne,
Batochime - Avenue Forel 2, 1015 Lausanne, Switzerland*

Ignacio Pagonabarraga*
*CECAM, Centre Européen de Calcul Atomique et Moléculaire,
EPFL, École Polytechnique Fédérale de Lausanne,
Batochime - Avenue Forel 2, 1015 Lausanne, Switzerland
Departament de Física de la Matèria Condensada,
Universitat de Barcelona, Martí i Franqués 1, 08028 Barcelona, Spain and
Universitat de Barcelona Institute of Complex Systems (UBICS),
Universitat de Barcelona, 08028 Barcelona, Spain*
(Dated: March 15, 2022)

## MODEL DETAILS

We present a mesoscopic model to simulate the dynamics of block copolymer nanocomposites with active Brownian particles. This hybrid in-grid/out-of-grid dynamic algorithm combines a continuous description for the BCP with an individual description of NPs following Brownian dynamics.

The total free energy of the system can be decomposed as

$$F_{tot} = F_{pol} + F_{cpl} + F_{cc} \tag{S1}$$

where the polymer free energy is $F_{pol}$, the coupling free energy $F_{cpl}$ introduces the presence of the NPs in the BCP, and the colloid-colloid interaction is $F_{cc}$.

### Block copolymer description

The BCP is characterized by the order parameter $\psi(\mathbf{r},t)$ which is related to the differences in the local monomer concentration $\phi_A(\mathbf{r},t)$ and $\phi_B(\mathbf{r},t)$ of block A and B, respectively,

$$\psi(\mathbf{r},t) = \phi_A(\mathbf{r},t) - \phi_B(\mathbf{r},t) + (1-2f_0) \tag{S2}$$

with the composition ratio $f_0 = N_A/(N_A+N_B)$ being the overall volume fraction of monomers A in the system. $\psi(\mathbf{r},t)$ is considered the local order parameter, which has a value 0 for the disordered-or homogeneous- state and $|\psi|>0$ for microphase-separated regions.

The time evolution of $\psi(\mathbf{r},t)$ is dictated by the conservation of mass, resulting in the Cahn-Hilliard-Cook equation [1–3]

$$\frac{\partial \psi(\mathbf{r},t)}{\partial t} = M\nabla^2 \left[\frac{\delta F_{tot}[\psi]}{\delta \psi}\right] + \eta(\mathbf{r},t) \tag{S3}$$

with $M$ being a mobility parameter and $\eta(\mathbf{r},t)$ being a gaussian noise parameter that satisfies the fluctuation-dissipation theorem

$$\langle \eta(\mathbf{r},t)\eta(\mathbf{r}',t')\rangle = -k_BTM\nabla^2\delta(\mathbf{r}-\mathbf{r}')\delta(t-t') \tag{S4}$$

for which we have used the algorithm given by Ball[3]. $k_BT$ sets the thermal energy scale of the diblock copolymer.

The polymeric free energy appearing in equation S1 is the standard Ohta-Kawasaki free energy[4], which can be further decomposed into short and long range terms $F_{pol} = F_{sr} + F_{lr}$ which can be expressed as

$$F_{\rm sr}[\psi] = \int d\mathbf{r}\left[H(\psi) + \frac{1}{2}D|\nabla\psi|^2\right] \tag{S5a}$$

$$F_{lr}[\psi] = \frac{1}{2}B\int d\mathbf{r}\int d\mathbf{r}' G(\mathbf{r},\mathbf{r}')\psi(\mathbf{r})\psi(\mathbf{r}') \tag{S5b}$$

with $G(\mathbf{r},\mathbf{r}')$ satisfying $\nabla^2 G(\mathbf{r},\mathbf{r}') = -\delta(\mathbf{r}-\mathbf{r}')$, i.e., the Green function for the Laplacian. The local free energy can be written as [5]

$$H(\psi) = \frac{1}{2}\tau'\psi^2 + \frac{1}{3}v(1-2f_0)\psi^3 + \frac{1}{4}u\psi^4 \tag{S6}$$

where $\tau' = -\tau_0 + A(1-2f_0)^2$, $u$ and $v$ specify the order parameter bulk values [4]. The local free energy $H(\psi)$ possesses 2 minima values $\psi_-$ and $\psi_+$ which are the values that $\psi(\mathbf{r},t)$ takes in the phase-separated domains. Parameter $D$ in Equation S5a is related to the interface size $\xi = \sqrt{D/\tau'}$ between domains and $B$ in Equation S5b to the periodicity of the system $H_0 \propto 1/\sqrt{B}$ as the long ranged free energy takes into account the junction of the two chains in a diblock copolymer.

### Block copolymer/nanoparticle coupling

The presence of $N_p$ number of particles in the BCP is introduced by a coupling term in the total free energy,

eq S1 as

$$F_{cpl} = \sum_{i=1...N_p} \sigma \int d\mathbf{r}\psi_c(\mathbf{r}-\mathbf{r}_i)\left[\psi(\mathbf{r})-\psi_0\right]^2 \tag{S7}$$

with a parameter $\sigma$ that controls the strength of the coupling interaction and an affinity parameter $\psi_0$ that specifies the selectivity of the colloidal particle with the BCP. The shape and size of the particle is determined by the tagged function $\psi_c(r < R) = exp\left[1 - 1/(1-(r/R)^2)\right]$ that decays monotonically and specifies the interior and exterior of the NP.

The colloid-colloid contribution to the free energy is introduced in eq. S1 as a pair-wise additive potential $F_{cc} = \sum_{j\neq i} V(r_{ij})$. The interparticle potential is chosen as a Yukawa-like potential that prevents overlapping between particles,

$$V(r_{ij}) = U_0\left[\frac{\exp(1-r/(2R))}{r/(2R)} - 1\right] \tag{S8}$$

where $U_0$ controls the strength of the interparticle potential.

## Active Brownian dynamics

The dynamics of $N_p$ active Brownian particles in the overdamped regime is controlled by the equations

$$\frac{d\mathbf{r}_i}{dt} = v_a\hat{\mathbf{n}}_i + \gamma_t^{-1}\left(\mathbf{f}_i^{cc} + \mathbf{f}_i^{cpl}\right) + \sqrt{2D_t}\xi_t \tag{S9a}$$

$$\frac{d\phi_i}{dt} = \gamma_r^{-1}\left(M_i^{cc} + M_i^{cpl}\right) + \sqrt{2D_r}\xi_r \tag{S9b}$$

where $\mathbf{r}_i$ and $\phi_i$ is the position and orientation of the $i$th particle, which includes a self-propulsion velocity $v_a$ with direction given by $\hat{\mathbf{n}}_i = (\cos\phi_i, \sin\phi_i)$. The diffusivity and friction for both the translational and orientational equations are related *via* the Einstein relation as $D_t = k_BT/\gamma_t$ and $D_r = k_BT/\gamma_r$ with $k_BT$ specifying the thermal state. Furthermore, the friction constants are related to the viscosity of the BCP $\eta_0$ as $\gamma_t = 6\pi\eta_0 R$ and $\gamma_r = 8\pi\eta_0 R^3$.

The forces acting on particle $i$ are of two kinds: coupling forces derived from the BCP medium, via the coupling free energy term equation S7 and the colloid-colloid repulsive forces that prevent overlapping, as shown in equation S8.

Additionally, we introduce aligning torques. The colloid-colloid torque promotes the alignment of particles within an interaction radius $R_{cc}$,

$$M_i^{cc} = \frac{K_{cc}}{\pi R_{cc}^2}\sum_{j\in\omega_i}\sin(\phi_i - \phi_j) \tag{S10}$$

where $K_{cc}$ controls the strength of the coupling interaction, while particle $i$ interacts with $\omega_i$ particles within a distance $r_{ij} < R_{cc}$. The range of the colloid-colloid alignment is chosen as twice the ABP diameter[6] $R_{cc} = 4R$.

The coupling of the colloid orientation and the BCP interface is achieved by introducing a torque term in which the orientation of particle $i$ is coupled with the gradient of the BCP field within a distance $R_{cpl} = R$ which is selected the same as the interaction of the colloid and the NP, as described in equation S7. The torque promotes the alignment of NPs along the interface, ie, it penalised the normal orientation of NPs at the interface, following

$$M_i^{cpl} = -\frac{K_{cpl}}{\pi R^2}\frac{\partial}{\partial\phi_i}\int d\mathbf{r}\left(\nabla\psi\cdot\hat{\mathbf{n}}_i\right)^2 \tag{S11}$$

where $K_{cpl}$ determines the strength of the coupling aligning interaction.

## Relevant dimensionless parameters

Given the large number of length, time and energy scales in the system, it is useful to list the relevant dimensional parameters and the consequent dimensionless parameters that will be used to set the appropiate regimes in the simulations.

### *BCP parameters*

The diffusive time scale can be extracted from the dynamic equation S3 as

$$t_{bcp} = \frac{L^2}{M\tau} \tag{S12}$$

where $L$ is the BCP length scale. The BCP possess two main length scales: the interface width $\xi_{iface}$ and the periodicity $H_0$. These two can be expressed as

$$\xi_{iface} = \sqrt{D/\tau} \tag{S13a}$$

$$H_0 = \alpha_0\sqrt{\tau/B} \tag{S13b}$$

where $\alpha_0$ is a numeric factor. The time scale associated to the polymer microphase separation is therefore

$$t_{bcp}^{iface} = \frac{\xi_{iface}^2}{\tau D} = \frac{D}{M\tau^2} \tag{S14}$$

which can be considered as the shortest time scale of the BCP dynamics. A secondary, slower dynamic scale can be similarly defined associated with the formation of the mesophase, ie, the lamellar or hexagonally-ordered circular phase.

The interaction between the BCP and the NP is dictated by the coupling free energy term, eq S7, therefore we can extract the energetic coupling scale as

$$\epsilon_{cpl} = \pi R^2 \sigma \tag{S15}$$

.

*ABP parameters*

The ABP dynamics can be characterised by a rotational and swimming time scale

$$t_{rot} = D_{rot}^{-1} = \frac{\gamma_{rot}}{k_B T} \tag{S16a}$$

$$t_{swim} = \frac{2R}{v_a} \tag{S16b}$$

where the rotational time scale quantifies the time for the NP to decorrelate from a given orientation, and the swimming time scale is the time that the NP requires to move a distance equal to its diameter. The NP-NP interaction strength is given by $U_0$ following equation S8, while the swimming energetic scale is

$$\epsilon_{swim} = v_a \gamma_{trans}(2R) \tag{S17}$$

The persistence length is the distance that the active particle moves without decorrelating its direction

$$l_{pers} = v_a t_{rot} \tag{S18}$$

In the absence of BCP coupling, the state of the purely ABP system is therefore specified by three dimensionless parameters

$$\phi_p = N_p \frac{\pi R^2}{L_x \times L_y} \tag{S19a}$$

$$Pe = \frac{t_{rot}}{t_{swim}} \tag{S19b}$$

$$\tilde{\epsilon}_{act} = \frac{\epsilon_{swim}}{U_0} \tag{S19c}$$

respectively, the surface fraction of the system occupied by colloids, the Peclet number comparing the rotational time scale versus the swimming time and the energetic swimming scale compared with the colloidal repulsion.

*Coupling dimensionless parameters*

The hybrid model for BCP/NP systems have been shown to possess several length, time and energetic scales. The comparison between them provides information regarding the regime in which the system is. The relative time scale between the colloidal swimming time and the polymer relaxation provides information regarding the ability of the BCP to accommodate a moving particle. We define a coupling Peclet-like number that compares the displacement time scale of the particle and the BCP microphase separation time scale

$$Pe^{cpl} = \frac{t_{bcp}}{t_{swim}} \tag{S20}$$

. In the regime in which $Pe^{cpl} \ll 1$ the BCP is able to accommodate the ABP displacement, while for $Pe^{cpl} \gg 1$ the swimming time is fast compared to the relaxation time of the BCP.

Similarly, quantifying the persistence length of the ABP with respect to the BCP length scales provides information regarding how the activity of the NP impacts the BCP morphology,

$$\tilde{l}_{pers} = \frac{l_{pers}}{L_{bcp}} \tag{S21}$$

where $L_{bcp}$ can refer to the most relevant length scale of the BCP, depending on the specific problem in play.

Additionally, we can compare the colloid swimming energetic scale with the energetic coupling with the BCP

$$\tilde{\epsilon}_{cpl} = \frac{\epsilon_{cpl}}{\epsilon_{swim}} \tag{S22}$$

. In a regime in which $\tilde{\epsilon}_{cpl} \gg 1$ the BCP-colloid coupling dominates over the active energetic scale, while for $\tilde{\epsilon}_{cpl} \ll 1$ the active energetic scale is large enough to allow the particle to escape the confinement imposed by the BCP, *eg*, the trapping of a neutral colloid at the interface, or the soft confinement induced by the domain walls for a selective colloid.

Finally, the orientational Brownian dynamics introduces two coupling torques corresponding to the colloid-colloid and the colloid-BCP alignment. Two dimensionless parameters can be defined that compare the characteristic alignment time and the diffusion rotational time

$$g_{cc} = \frac{K_{cc}}{\pi R_{cc}^2 k_B T} \tag{S23a}$$

$$g_{cpl} = \frac{K_{cpl}}{\pi R^2 k_B T} \tag{S23b}$$

which correspond to the relative strength of the colloid-colloid and the colloid-BCP coupling torques, respectively. The calibration of these parameters are shown in figure S1 **B** and **C**.

### Observables

We make use of several magnitudes to study the configuration of the overall system. For sake of clarity we list the observables that are used throughout this work.

The degree of microphase separation of the BCP can be roughly quantified with the mean absolute value of the BCP field $< |\psi| >$ which takes a value $< |\psi| > \ll 1$ for a homogeneous disordered state and a $\sim 1$ value for a phase separated regime. This magnitude is extensively used to determine the equilibration of the BCP time evolution.

The fraction of particles located at the interface is given by the ratio $\Phi = N_{interface}/N_p$. The fraction of NPs at the interface is determined by calculating the average value of the BCP concentration field $\psi$ in the vicinity of the NP surface.

Out of the particles considered within the interface we determine the nematic-like coupling order parameter

$$S_{cpl} = \frac{1}{N_{interface}} \sum_{i=1}^{N_{interface}} 2\left(\hat{\mathbf{n}}_i \cdot \hat{\mathbf{P}}\right)^2 - 1 \tag{S24}$$

where $\hat{\mathbf{P}}$ is the local BCP orientation, given by an average of the gradient of the order parameter $\hat{\mathbf{P}} \propto \nabla\psi(\mathbf{r})$

Due to the lack of global nematic or polar ordering, we define orientational parameters locally, with each particle possessing orientational ordering with respect to immediate neighbors. The mean polarisation of the ABP is calculated as the average over all particles, with each particle polarisation defined with respect to immediate neighboring particles as

$$P_{cc} = \frac{1}{N_p} \sum_{i=1}^{N_p} \frac{1}{N_i} \sum_{j=1}^{N_i} \hat{\mathbf{n}}_i \cdot \hat{\mathbf{n}}_j \tag{S25}$$

where $N_i$ is the number of first neighbors within a distance $r_{ij} < r^*_{ij}$ of particle $i$, with $r^*_{ij} = 1.3(2R)$ the cutoff determined from the radial distribution function. The mean polarisation is useful to determine instances of collective swarm or cluster formation with coherent internal polarisation.

A similar procedure is used to determine the relative nematic order between particles with respect to the interparticle distance

$$S_{rel} = \frac{1}{N_p} \sum_{i=1}^{N_p} \frac{1}{N_i} \sum_{j=1}^{N_i} 2\left(\hat{\mathbf{r}}_{ij} \cdot \hat{\mathbf{n}}_j\right)^2 - 1 \tag{S26}$$

where $\hat{\mathbf{r}}_{ij} = (\mathbf{r}_i - \mathbf{r}_j)/|\mathbf{r}_i - \mathbf{r}_j|$ is the unit vector between particle's center of mass.

In order to get insight over the morphology of the ABP clusters, we perform cluster analysis to determine the cluster size distribution. Particles are considered to belong to a cluster via the interparticle distance $r_{ij} < r^*_{ij} = 1.3(2R)$. We analyse the shape of the clusters by calculating the number of neighbors per particle, after selecting all clusters with a size larger than 3 ABPs. Clusters with a 1D shape are considered if all the particles belonging to the cluster have two immediate neighbors, apart from particles in the extremes of the cluster. Finally, the fraction of 1D clusters is determined as

$$\Phi_{1D} = \frac{\text{1D-like clusters}}{\text{Clusters with} > 3 \text{ ABPs}} \tag{S27}$$

The angular frequency of the chiral motion of ABPs $\omega_c$ is determined for each ABP cluster via the angular momentum

$$\mathbf{L}_c = \sum_i \mathbf{r} \times \mathbf{v}_i \rightarrow \mathbf{L}_c = I_c \omega_c \tag{S28}$$

for all particles $i$ belonging to cluster $c$. The tensor $I_c$ is the moment of inertia tensor, which we determine for each cluster $c = 1...N_c$ for $N_c$ number of clusters (we neglect clusters with less than $N^*_c = 4$ particles). The mean absolute value of the angular frequency $\langle|\omega_c|\rangle$ along all clusters is used to quantify the chirality of the ABP motion.

Finally, the BCP morphology is analysed via domain analysis to determine the shape of the domains. The fraction of circular domains $\Phi^{BCP}_{circle}$ over the total number of domains takes a value $\sim 1$ in the circular phase.

## ADDITIONAL PARAMETERS

In this work we use standard parameters used for cell dynamic simulations $\tau = 0.35$, $u = 0.5$, $v = 1.5$ , $A = 1.5$, $D = 1.0$ and $B = 0.0002$. For symmetric lamellar-forming BCP (figure 1) $f_0 = 0.5$ and for circle-forming asymmetric BCP $f_0 = 0.3$.

### Details on simulation initialisation

For clarity, we list the initial condition on each of the figures in the main text and the rationale for its choice: In general, we select a random initial state for the lamellar-forming BCP, and an equilibrated initial condition for the cicle-forming BCP.

In **figure 1** we consider a lamellar-forming BCP. In experiments or simulations, lamellar-forming BCP rarely self-assembles into globally ordered equilibrium morphologies without defects, unless external fields are applied. For this reason, it would be unrealistic to initialise the system from an equilibrated state. Instead, we consider an initial random distribution of BCP melt $\psi$ that emulates a rapid quench from disorder into order morphology. On the other hand, the ABPs are also randomly assigned positions and orientations at $t = 0$.

For **figures 2,3,4 and 5** we consider an initially ordered BCP phase which is obtained from a previous simulation run with no particles. The rationale for this choice is that the hexagonally ordered circles phase is rapidly obtained in asymmetric BCP melts without the need of external fields. Furthermore, ABPs are initially placed at the interface to facilitate the segregation into their preferred domains (either the interface for neutral particles, or the interior of the circular domains for selective ones). The orientation of the ABPs is always random. Figure S3 compares the result from figure 3 by choosing a random initial condition. This is motivated by the fact that the

## ACTIVE BROWNIAN PARTICLES IN SUSPENSION: CALIBRATION

In figure S1 we calibrate some of the parameters. In **A** we can observe the expected motility-induced phase separation behaviour for ABPs in the absence of medium. In **B** and **C** we calibrate the nematic alignment and polarisation of the aligning torques, respectively, in terms of the dimensionless parameters defined in the main text.

## NEUTRAL, DILUTE PARTICLES IN ADDITIONAL BCP MORPHOLOGIES

Figure 1 has shown the orientation and interface behaviour of the ABP in a lamellar-forming BCP in the absence of orieantional coupling, *ie* $g_{cc} = g_{cpl} = 0$ in equations S23a and S23b. In this section we explore the coupling orientation $S_{scpl}$ in a circular and defect-free lamellar morphology, in figure S2. In a defect-free lamellar BCP morphology the BCP interfaces possess zero curvature which, following the argument used in the main text, limits the tendency of ABP to get stuck for a time $t_{rot}$ in a high-curvature region. For this reason, in a defect-free lamellar morphology $S_{cpl} \leq 0$, *ie* there are no instances of normal orientation of ABP with respect to the interface. On the other hand, circular-forming BCP possess intrinsic curvature which leads to a slight increase in the maximum value of $\max(S_{cpl}) \sim 0.15$, above the maximum value observed in figure 1 **A**. Following a similar argument, the intrinsic curvature of the BCP morphology promotes the particle to remain within a region of the interface in which the orientation of the ABP is normal to the interface, for a time $t_{rot}$, before decorrelating its orientation and moving elsewhere. The comparison between figure 1 and the two curves in S2 highlights the role of the BCP morphology in the configuration of the ABP, even in the extremely simple case of ABP without orientational coupling with the BCP or with themselves.

* ipagonabarraga@ub.edu

[1] J. W. Cahn, The Journal of Chemical Physics **30**, 1121 (1959).
[2] H. E. Cook, Acta Metallurgica **18**, 297 (1970).
[3] R. C. Ball and R. L. H. Essery, Journal of Physics: Condensed Matter **2**, 10303 (1990).
[4] T. Ohta and K. Kawasaki, Macromolecules **19**, 2621 (1986), publisher: American Chemical Society.
[5] I. W. Hamley, Macromolecular Theory and Simulations **9**, 363 (2000).
[6] E. Sesé-Sansa, I. Pagonabarraga, and D. Levis, EPL (Europhysics Letters) **124**, 30004 (2018).

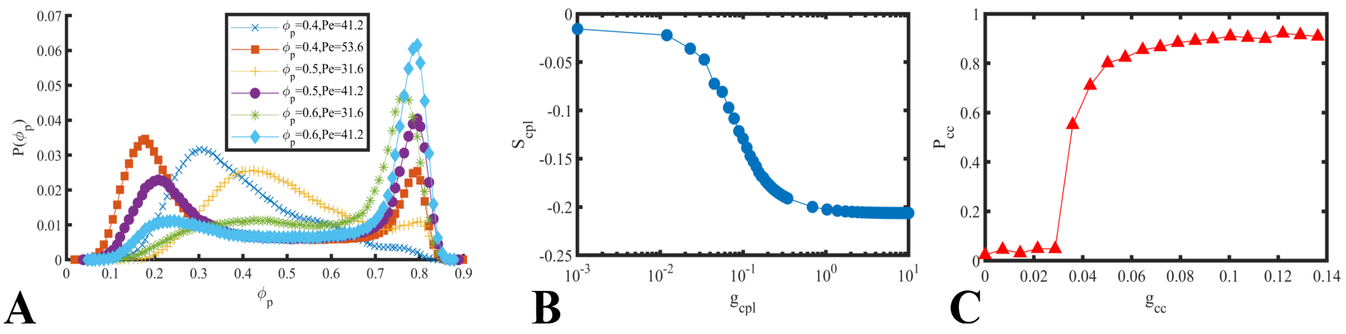


Figure S1. **A** Probability distribution function of local volume fraction $\phi_p$ for several values of the Peclet number $Pe$ and the overall volume fraction $\phi_p$. The location of the transition from unimodal to bimodal curves is in accordance with MIPS boundaries in ABP. **B**. **C** Global polarisation with $\phi_p = 0.4$ and $Pe = 30$.

| filename | $Pe$ | $\phi_p$ | figure | notes |
|---|---|---|---|---|
| `phase-I.mp4` | 0.2 | 0.01 | 1 | passive-like |
| `phase-II.mp4` | 2.8 | 0.01 | 1 | $S_{cpl} > 0$, interface |
| `phase-III.mp4` | 38.6 | 0.01 | 1 | $S_{cpl} < 0$, escaped |
| `neutral-phase-I_Pe1.mp4` | 1 | 0.05 | 2 | passive-like |
| `neutral-phase-II_Pe8.mp4` | 8 | 0.05 | 2 | disordered clusters |
| `neutral-phase-III_Pe22.mp4` | 22 | 0.05 | 2 | polarised trains |
| `neutral-phase-IV_Pe100.mp4` | 100 | 0.05 | 2 | swarms |
| `selective_phase-I.mp4` | 0.2 | 0.06 | 4 | passive-like |
| `selective_phase-II.mp4` | 12 | 0.06 | 4 | polarised trains |
| `selective_phase-III.mp4` | 2.3 | 0.15 | 4 | disordered clusters |
| `selective_phase-IV.mp4` | 140 | 0.12 | 4 | swarms |

Table I. Summary of supplementary files (videos) and the corresponding figure in the main text

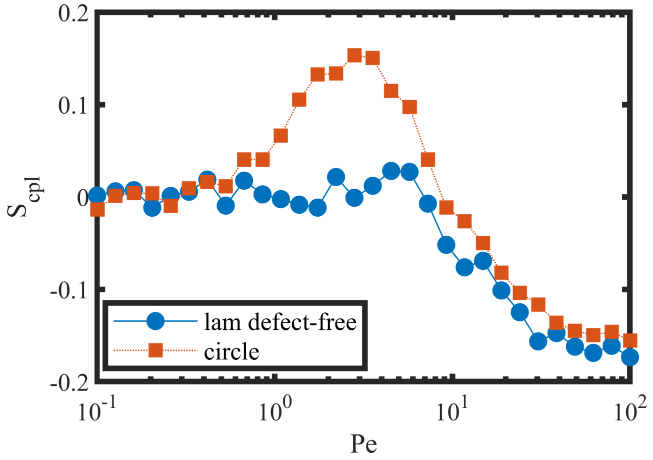


Figure S2. Nematic-like order parameter in dependence of the $Pe$ Peclet number for a lamellar-forming BCP with no defects and a circular-forming BCP.

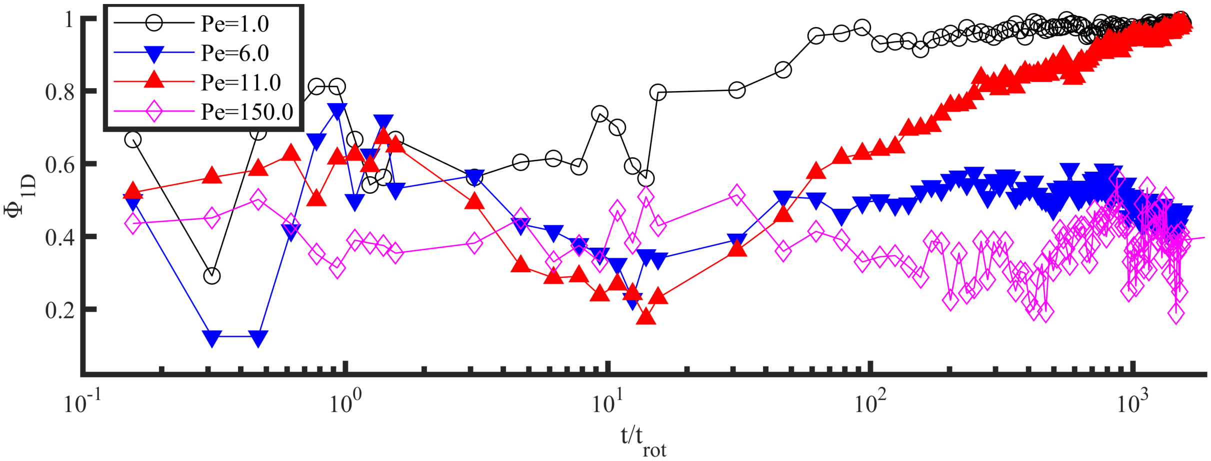


Figure S3. **Dynamic behaviour of the fraction of 1D NP clusters** for four representative activities corresponding to the four regimes identified in figure 2. The system is initialised from a disordered state: a homogeneous melt for the BCP, and a random distribution of ABPs (translation and orientation) . It can be compared with figure 3 in the main text for an initially-ordered system.

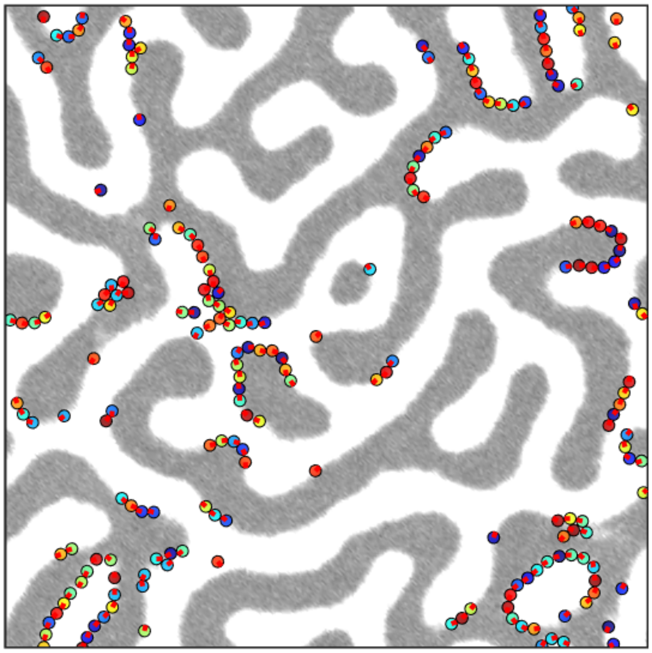

Figure S4. Polarised train regime formed by 1D clusters of neutral articles in lamellar-forming BCP. All parameters are the same as in figure 2 of the main text for $Pe = 22$, $\phi_p = 0.05$, expect $f_0 = 1/2$, *i.e.* symmetric BCP phase.

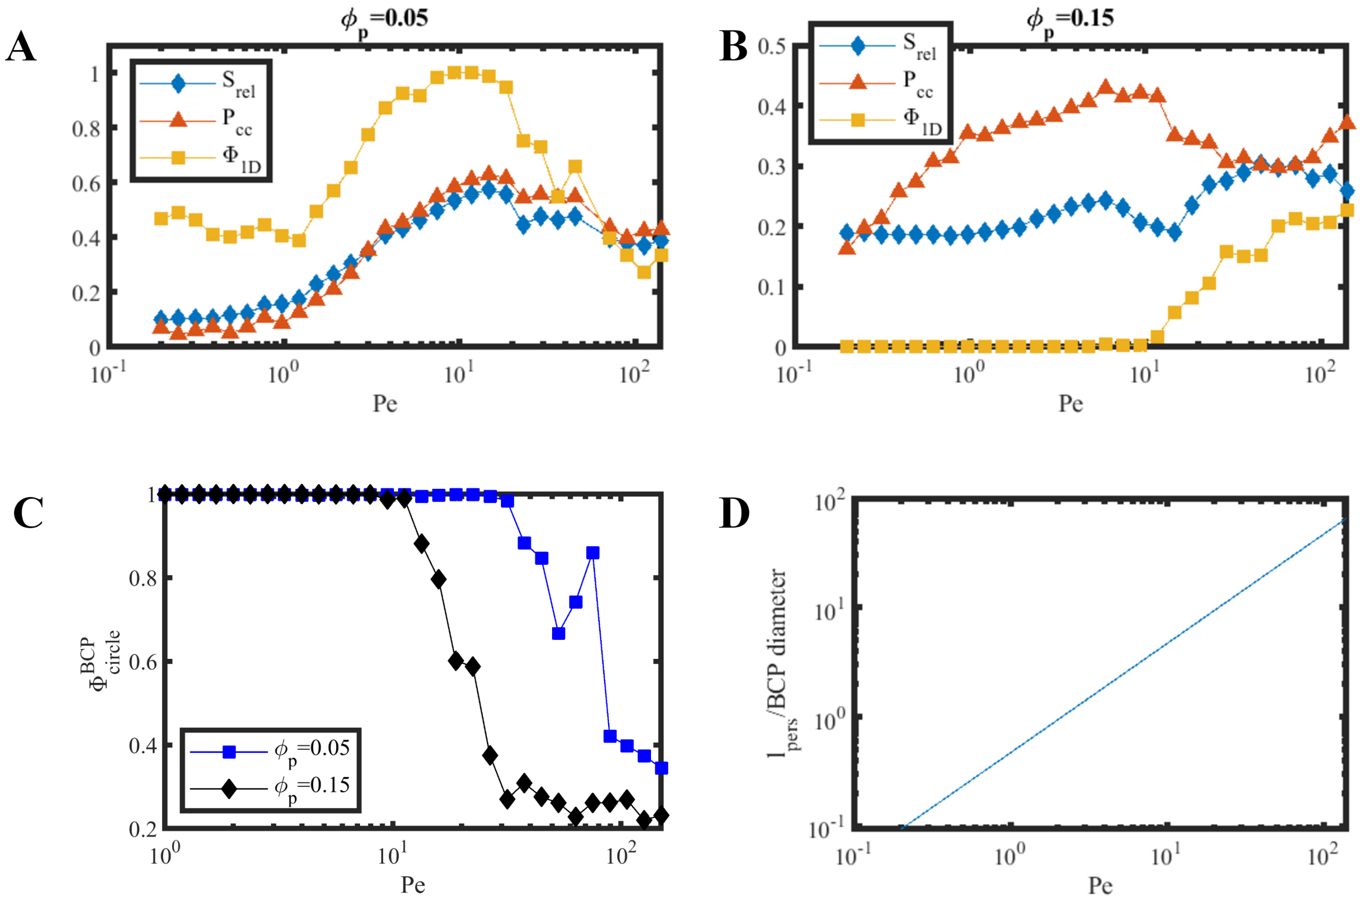


Figure S5. Observables used to determine the various regimes in figure 4 of the main text, for selective ABPs with $\psi_0 = -1$. Two concentrations are considered $\phi_p = 0.05$ and $\phi_p = 0.15$ which span across the four regimes of the phase diagram for different values of the $Pe$. The persistence length $l_{pers}$ is compared with the radius of the BCP domains to estimate the activity at which the particles' self-propel encountering a BCP domain wall.
